# Supplementary material for: An Offline Meta Black-box Optimization Framework for Adaptive Design of Urban Traffic Light Management Systems
Source: arXiv:2408.07327 source file (2024-08-14)
Supplement: Supplementary file 1 [file extra_figure.tex]

\section{Extra Figures}\label{app:extra_figure}
In this section, we visualize extra experiment results that are not presented in the main paper due to page limits. We plot the performance of our proposed method and meta black-box optimization methods over the course of the evaluation. The figures show that our method consistently outperforms baselines and demonstrates fast convergence to optimal design. 
\begin{table}[h]
\centering
\caption{Details on optimized traffic signals in District A}
\vspace{-7pt}
\resizebox{\linewidth}{!}{
\begin{tabular}{c|ccc}
\toprule
 \textbf{Intersection ID} & \# of Phases & Min Green Time & Cycle Time\\
\midrule
1	&	3	& 75/36/34 & 160\\
2	&	4	& 79/18/30/18	&	160\\
3	&	4	& 74/18/34/18	&	160\\
4	&	4	& 64/17/31/31	&	160\\
5	&	4	& 84/17/13/30 & 160\\
6	&	4	& 61/17/38/29 & 160\\
7	&	4	& 71/18/28/28 & 160\\
8	&	4	& 71/18/28/28 & 160\\
9	&	4	& 27/70/16/32 & 160\\
10	&	5	& 22/47/34/24/17 & 160\\
11	&	3	& 69/10/38 & 130\\
12	&	3	& 63/21/33 & 130\\
13	&	3	& 60/35/22 & 130\\
14	&	4	& 48/44/44/31 & 185\\
15	&	3	& 126/22/18 & 185\\
16	&	3	& 48/24/27 & 110\\
17	&	5	& 57/49/18/25/13 & 180\\
18	&	4	& 80/40/28/13 & 180\\
19	&	3	& 115/18/29 & 180\\
20	&	5	& 27/36/41/21/36 & 180\\
21	&	5	& 45/45/21/26/26 & 180\\
22	&	5	& 45/40/21/27/29 & 180\\
23	&	5	& 54/38/16/27/26 & 180\\
24	&	5	& 33/35/36/30/29 & 180\\
25	&	5	& 48/37/12/35/30 & 180\\
26	&	3	& 74/27/62 & 180\\
\bottomrule
\end{tabular}}
\label{table:districtA_info}
\end{table}
\clearpage
\begin{figure*}[t]
\begin{minipage}[t]{0.8\textwidth}  
    \begin{subfigure}[t]{0.45\textwidth}
         \includegraphics[width=\textwidth]{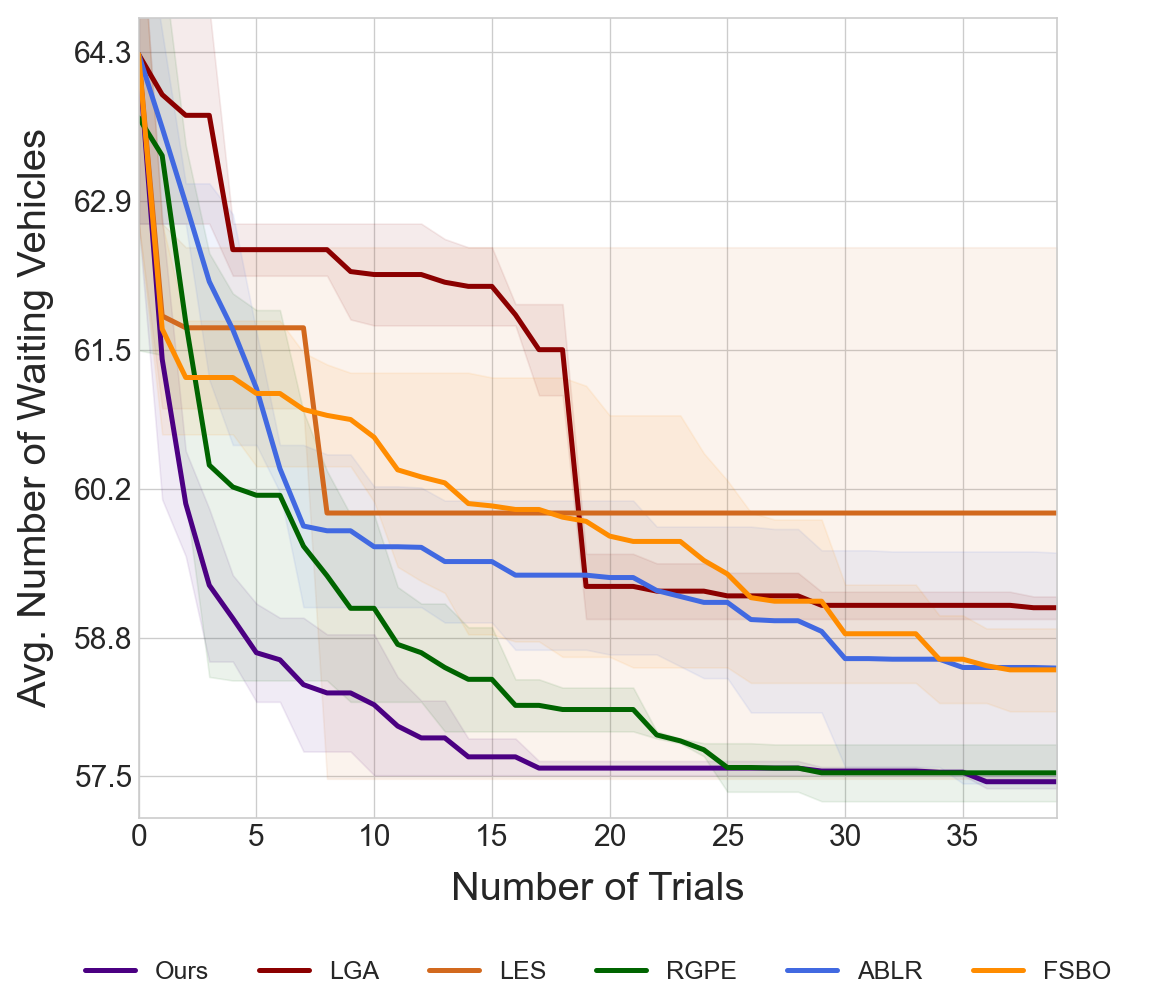}
         \caption{Phase combination}
     \end{subfigure}
     \begin{subfigure}[t]{0.45\textwidth}
        \includegraphics[width=\textwidth]{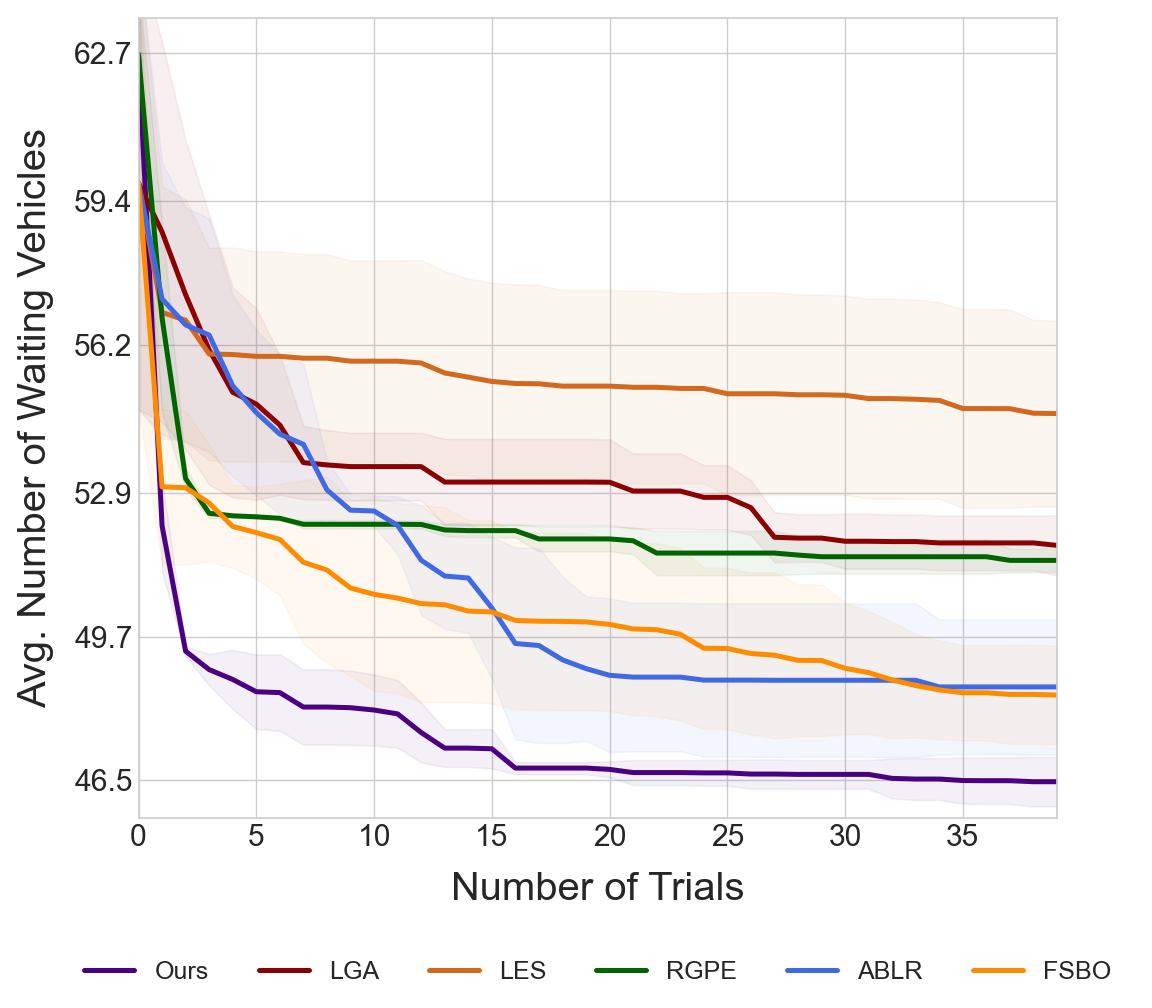}
         \caption{Phase allocation}
     \end{subfigure}     
\end{minipage} 
\caption{Experiments on Grid 2$\times$2 network}\label{figure:2by2}
\end{figure*}

\begin{figure*}[t]
\centering
\begin{minipage}[t]{0.8\textwidth}  
    \begin{subfigure}[t]{0.45\textwidth}
         \includegraphics[width=\textwidth]{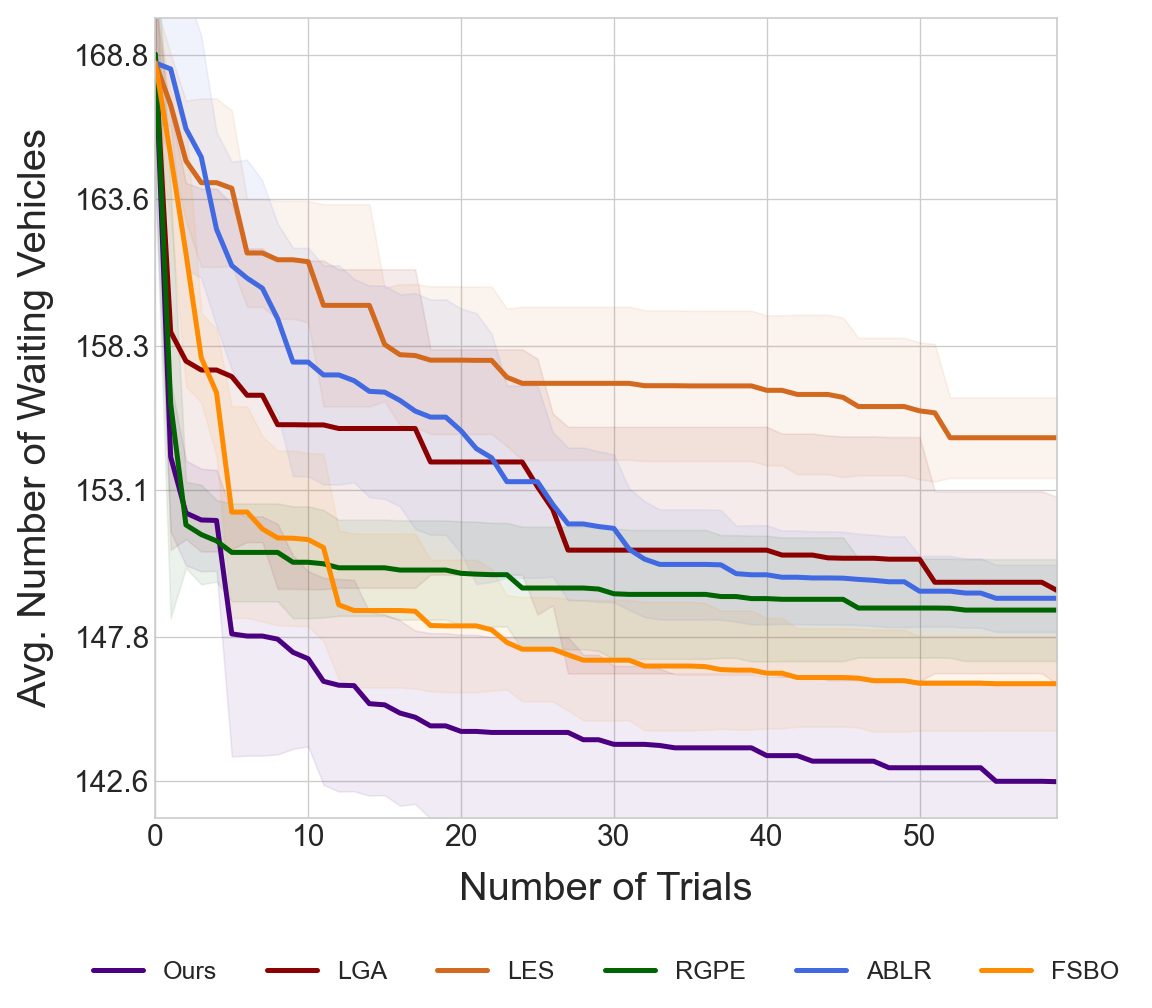}
         \caption{Phase combination}
     \end{subfigure}
     \begin{subfigure}[t]{0.45\textwidth}
        \includegraphics[width=\textwidth]{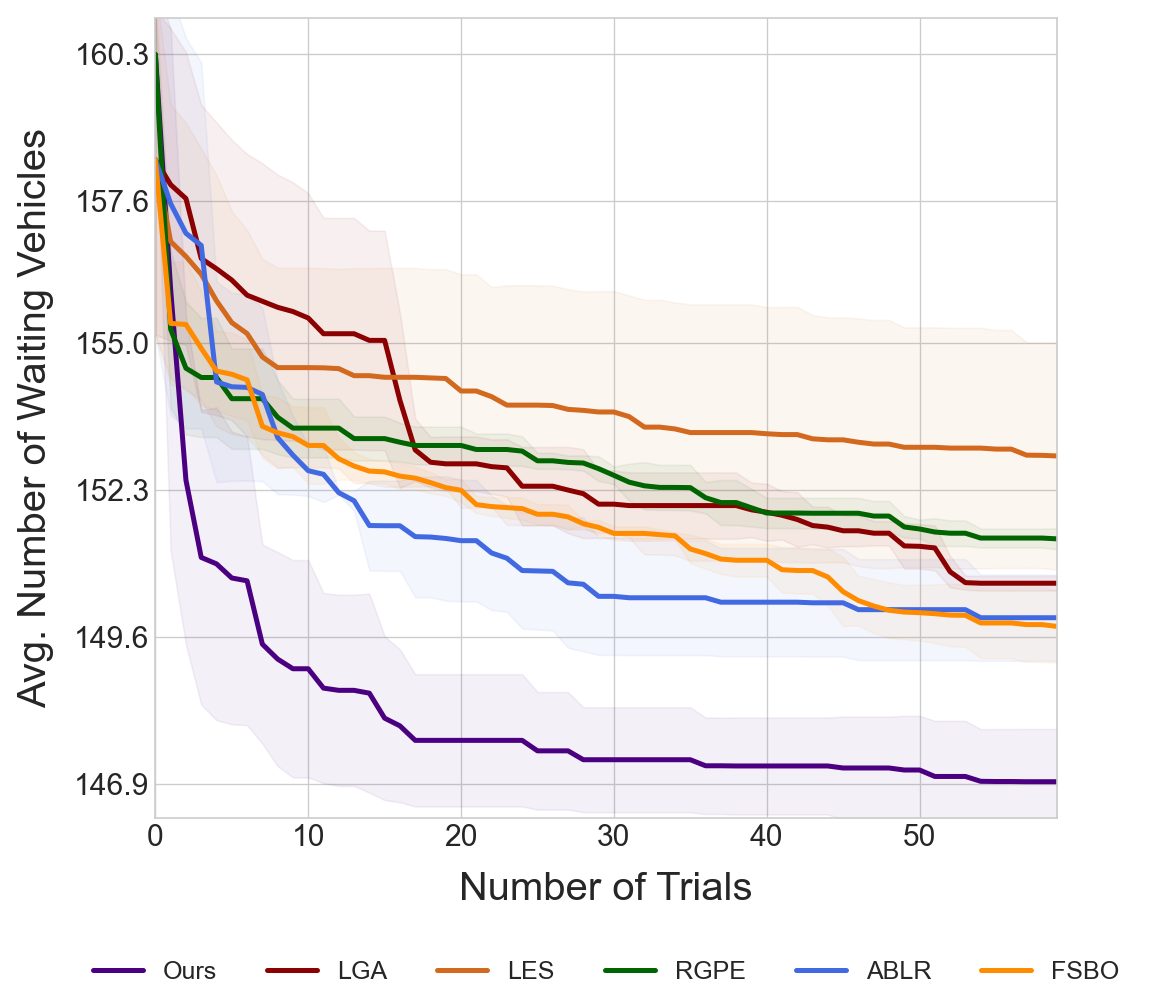}
         \caption{Phase allocation}
     \end{subfigure}     
\end{minipage} 
\caption{Experiments on Grid 3$\times$3 network}\label{figure:3by3}
\end{figure*}

\begin{figure*}[t]
\centering
\begin{minipage}[t]{0.8\textwidth}  
    \begin{subfigure}[t]{0.45\textwidth}
         \includegraphics[width=\textwidth]{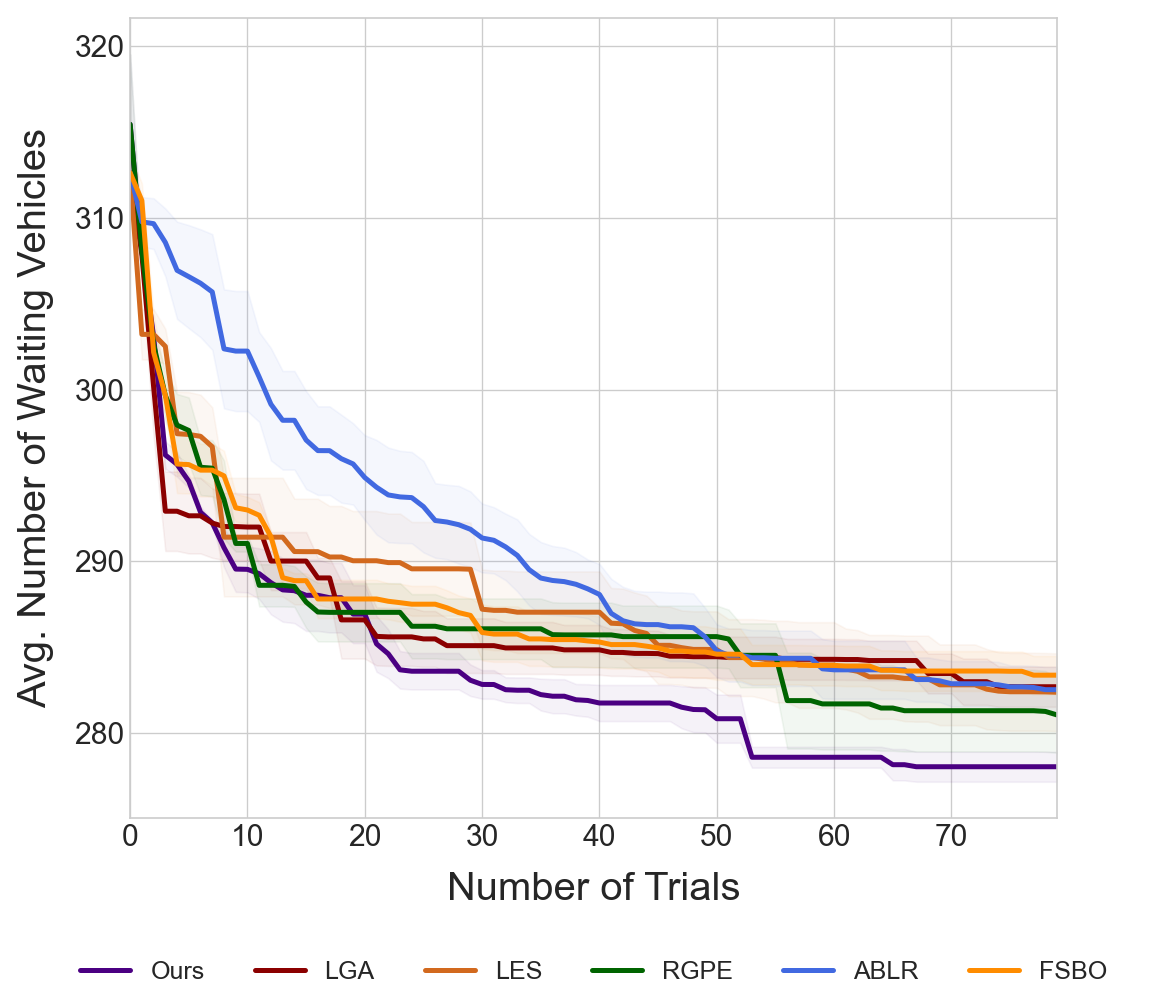}
         \caption{Phase combination}
     \end{subfigure}
     \begin{subfigure}[t]{0.45\textwidth}
        \includegraphics[width=\textwidth]{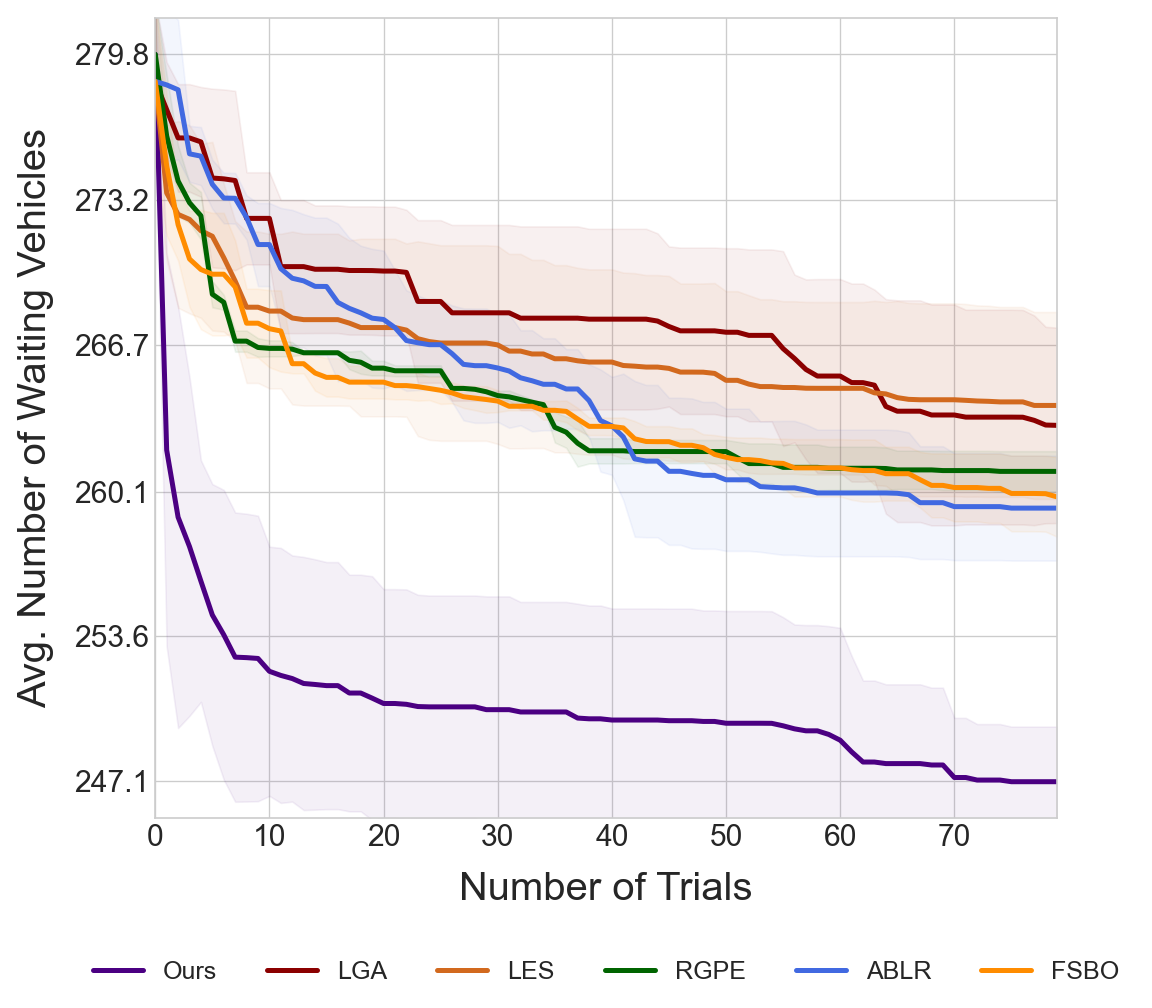}
         \caption{Phase allocation}
     \end{subfigure}     
\end{minipage} 
\caption{Experiments on Grid 4$\times$4 network}\label{figure:4by4}
\end{figure*}

\begin{figure*}[t]
\centering
\begin{minipage}[t]{0.8\textwidth}  
    \begin{subfigure}[t]{0.45\textwidth}
         \includegraphics[width=\textwidth]{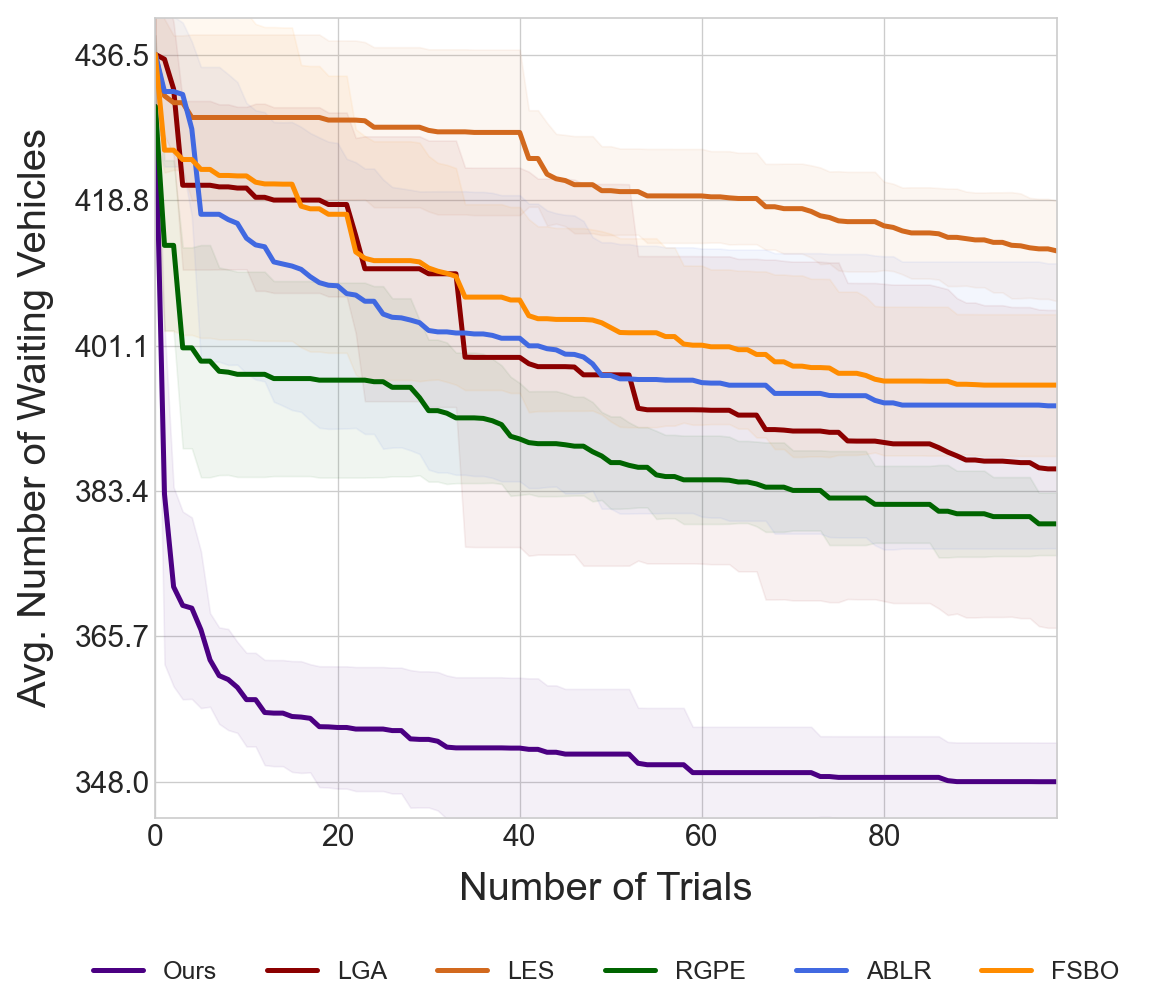}
         \caption{Phase combination}
     \end{subfigure}
     \begin{subfigure}[t]{0.45\textwidth}
        \includegraphics[width=\textwidth]{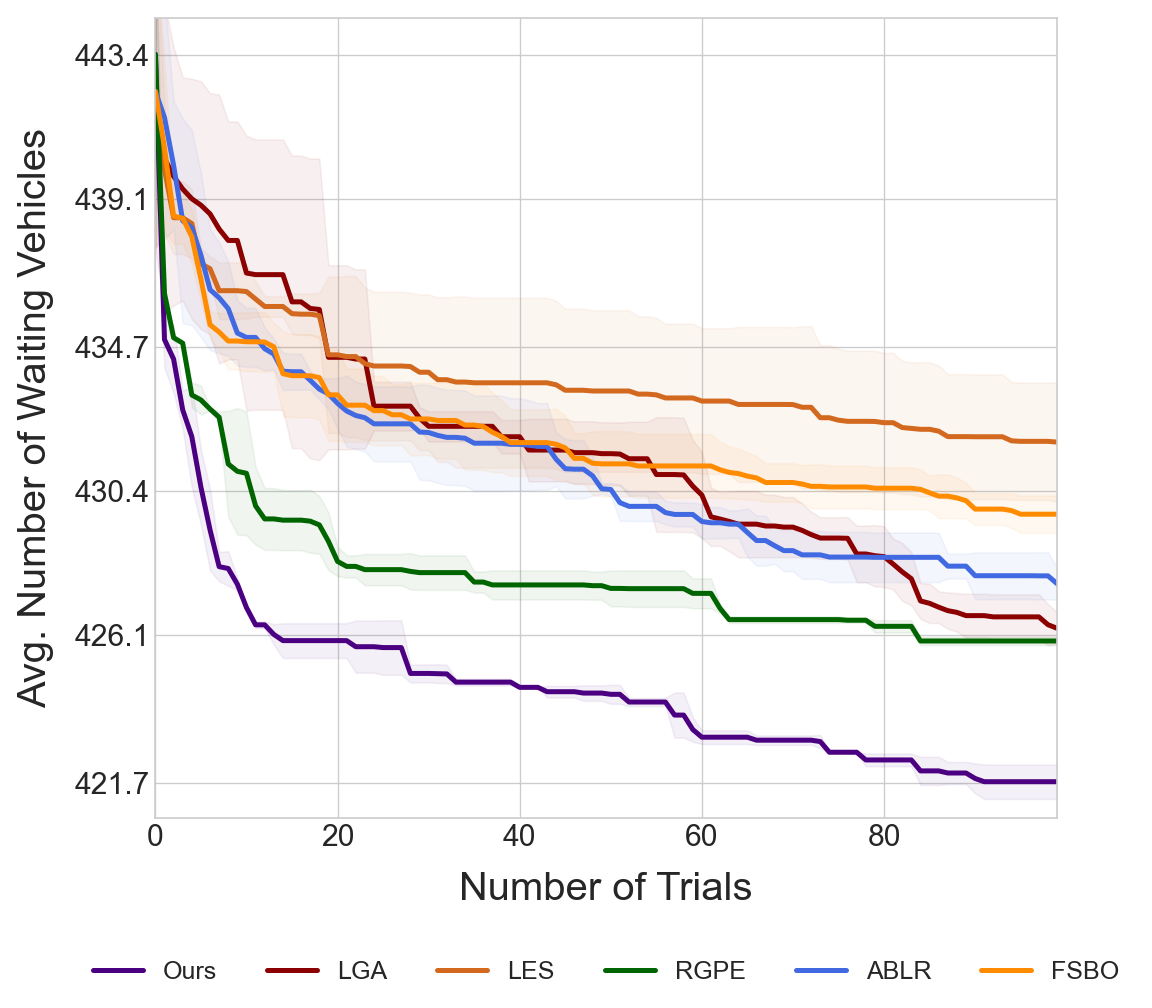}
         \caption{Phase allocation}
     \end{subfigure}     
\end{minipage} 
\caption{Experiments on Grid 5$\times$5 network}\label{figure:5by5}
\end{figure*}

% \begin{figure*}[t]
% \centering
% \begin{minipage}[t]{0.8\textwidth}  
%     \begin{subfigure}[t]{0.45\textwidth}
%          \includegraphics[width=\textwidth]{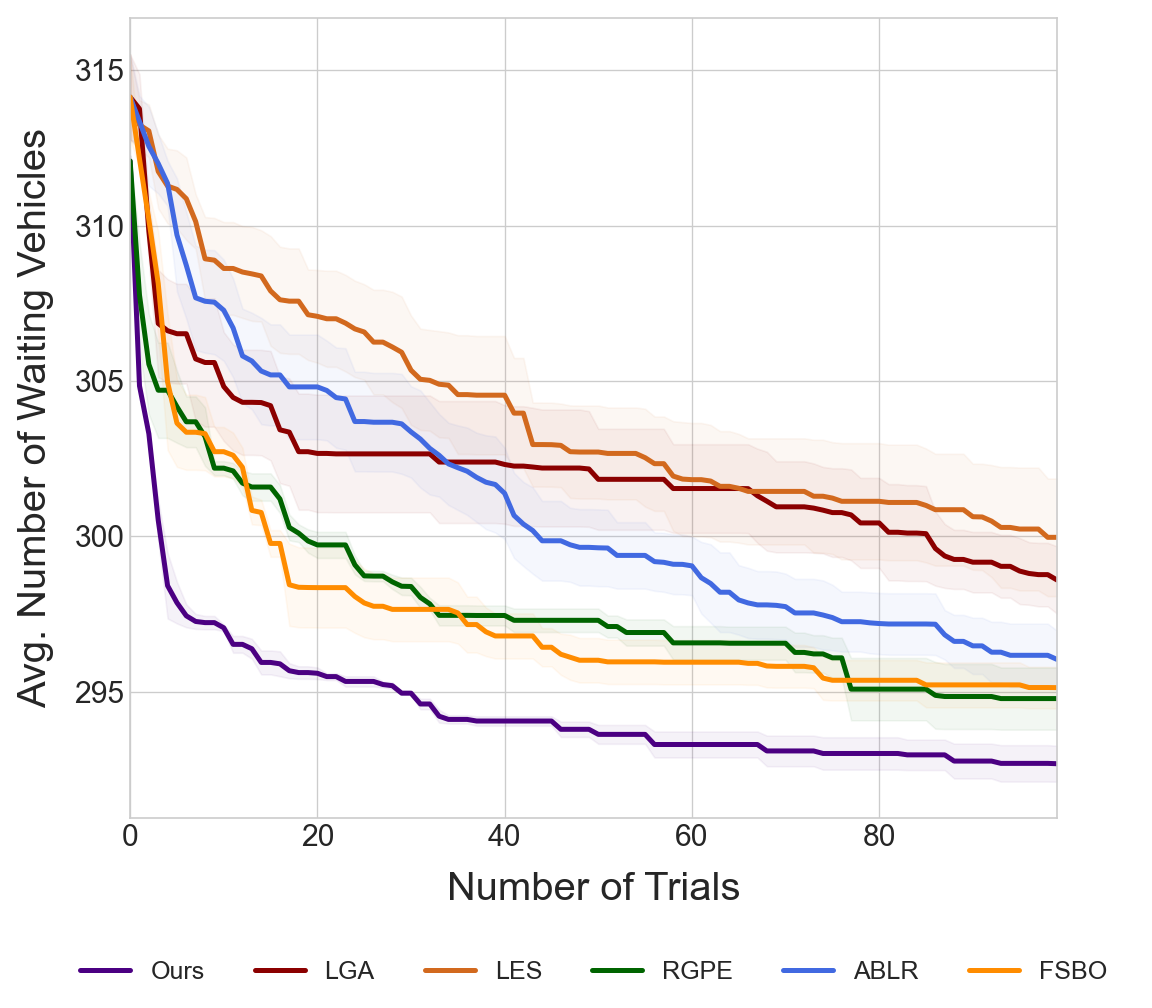}
%          \caption{Phase combination}
%      \end{subfigure}
%      \begin{subfigure}[t]{0.45\textwidth}
%         \includegraphics[width=\textwidth]{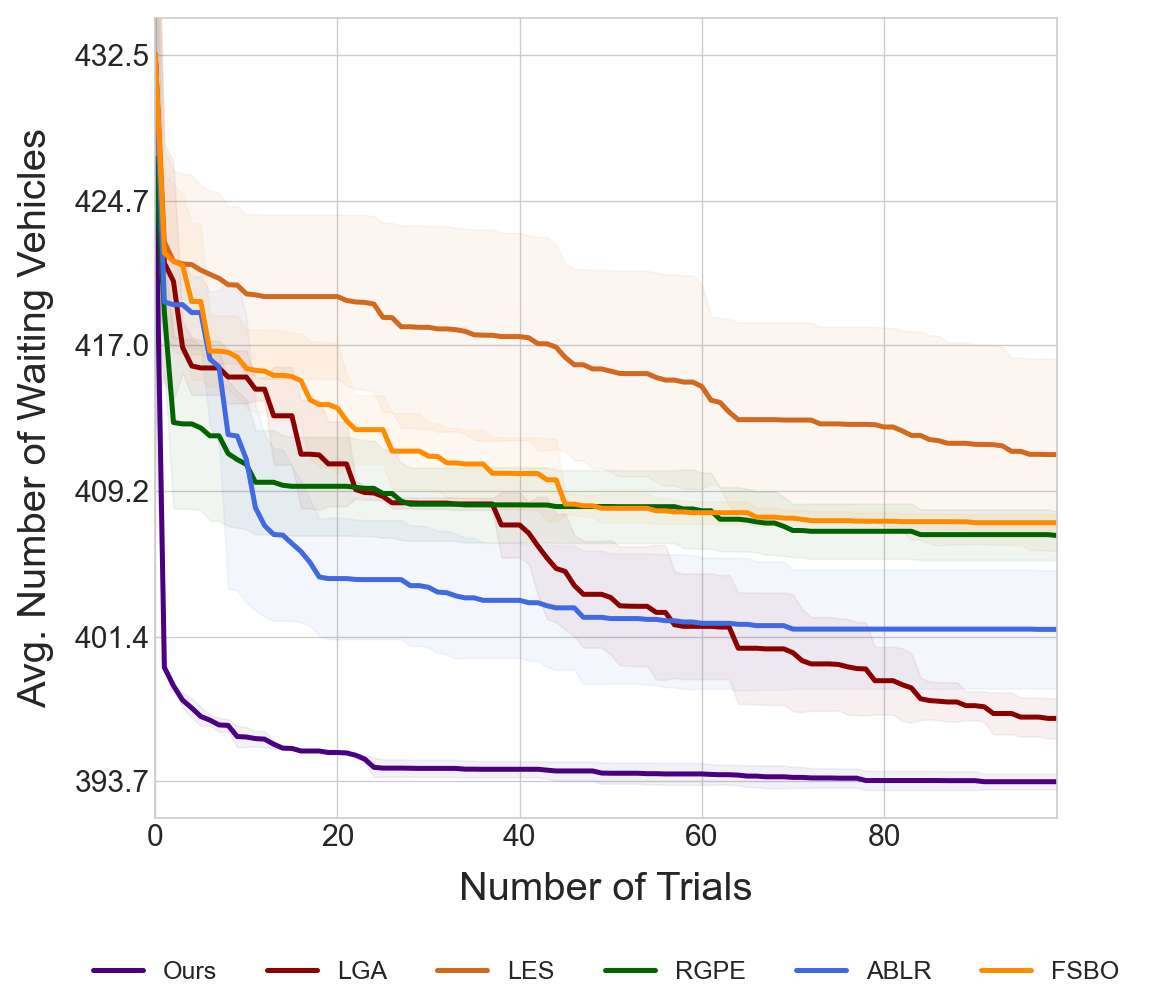}
%          \caption{Phase allocation}
%      \end{subfigure}     
% \end{minipage} 
% \caption{Experiments on Hangzhou 4$\times$4 network}\label{figure:hangzhou}
% \end{figure*}

\begin{figure*}[t]
\centering
\begin{minipage}[t]{0.8\textwidth}  
    \begin{subfigure}[t]{0.45\textwidth}
         \includegraphics[width=\textwidth]{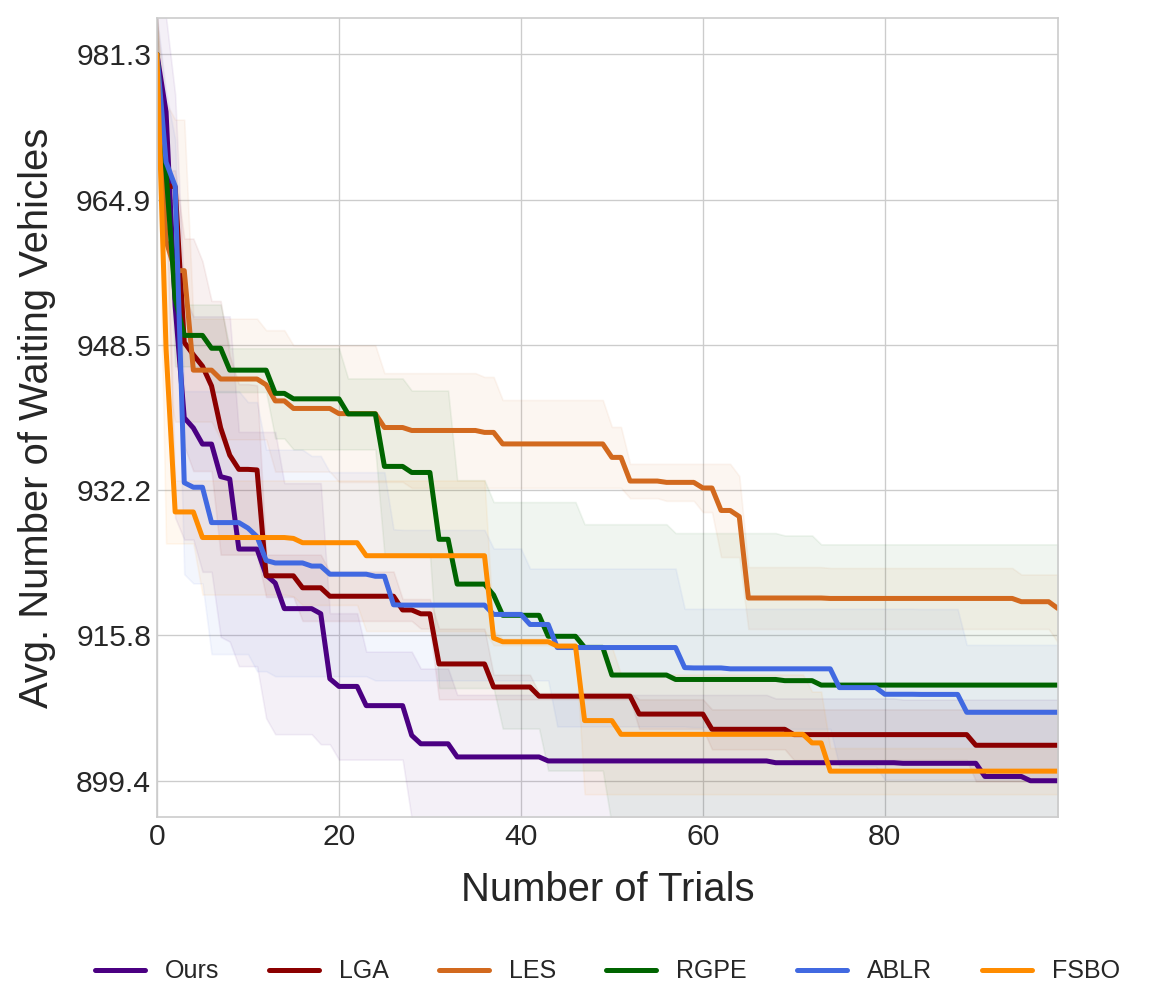}
         \caption{Phase combination}
     \end{subfigure}
     \begin{subfigure}[t]{0.45\textwidth}
        \includegraphics[width=\textwidth]{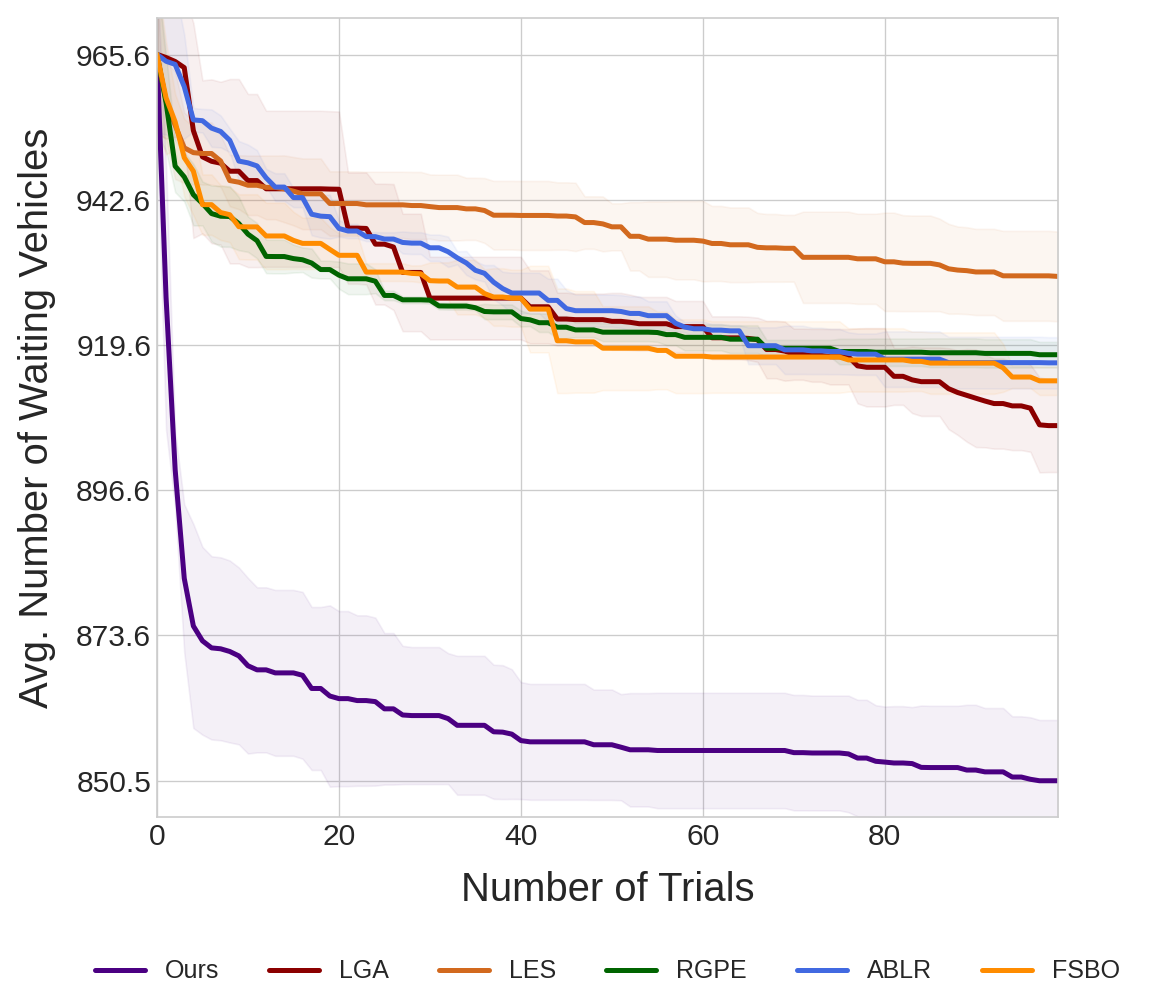}
         \caption{Phase allocation}
     \end{subfigure}     
\end{minipage} 
\caption{Experiments on Manhattan 16$\times$3 network}\label{figure:manhattan}
\end{figure*}

\begin{figure*}[t]
\centering
\begin{minipage}[t]{0.8\textwidth}  
    \begin{subfigure}[t]{0.45\textwidth}
         \includegraphics[width=\textwidth]{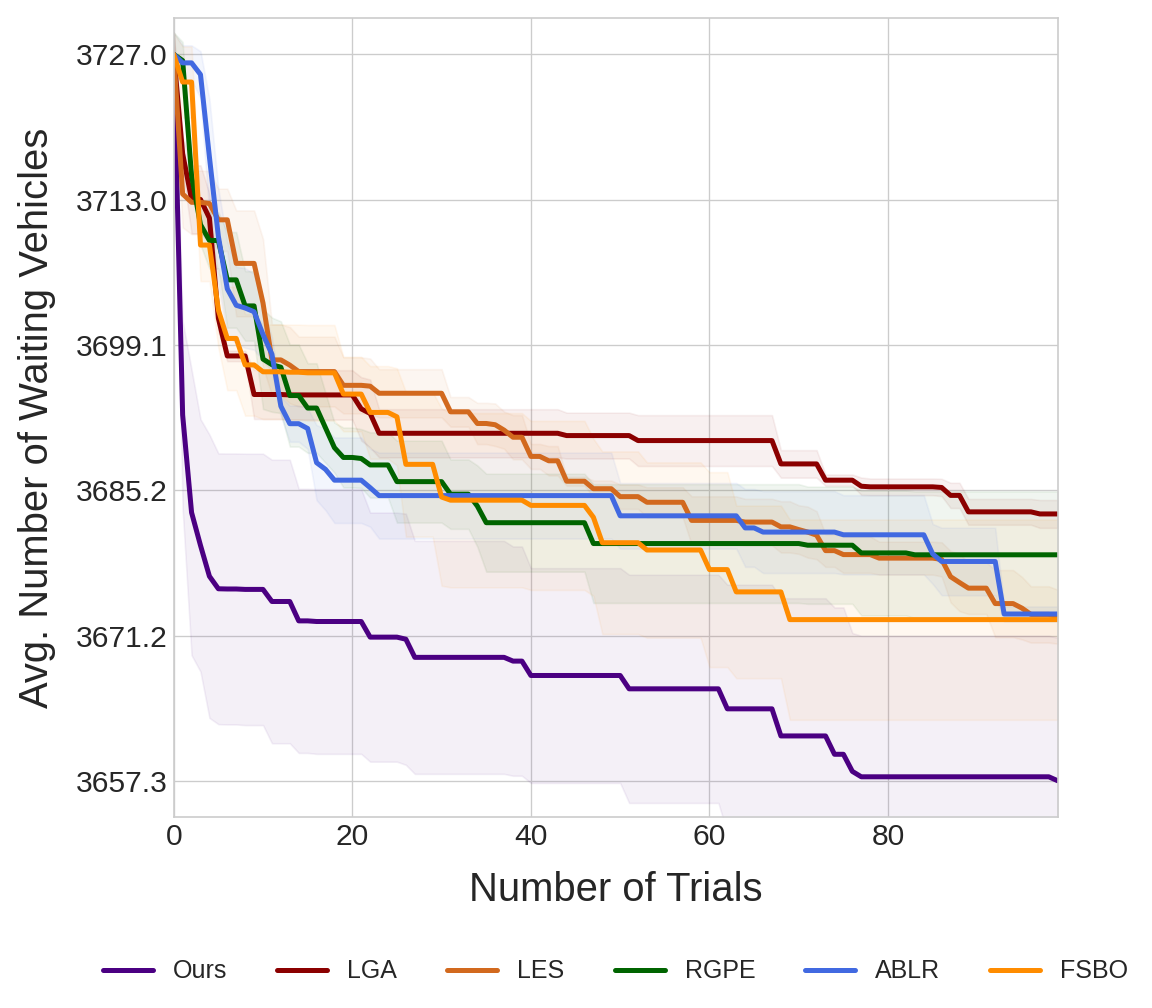}
         \caption{Phase combination}
     \end{subfigure}
     \begin{subfigure}[t]{0.45\textwidth}
        \includegraphics[width=\textwidth]{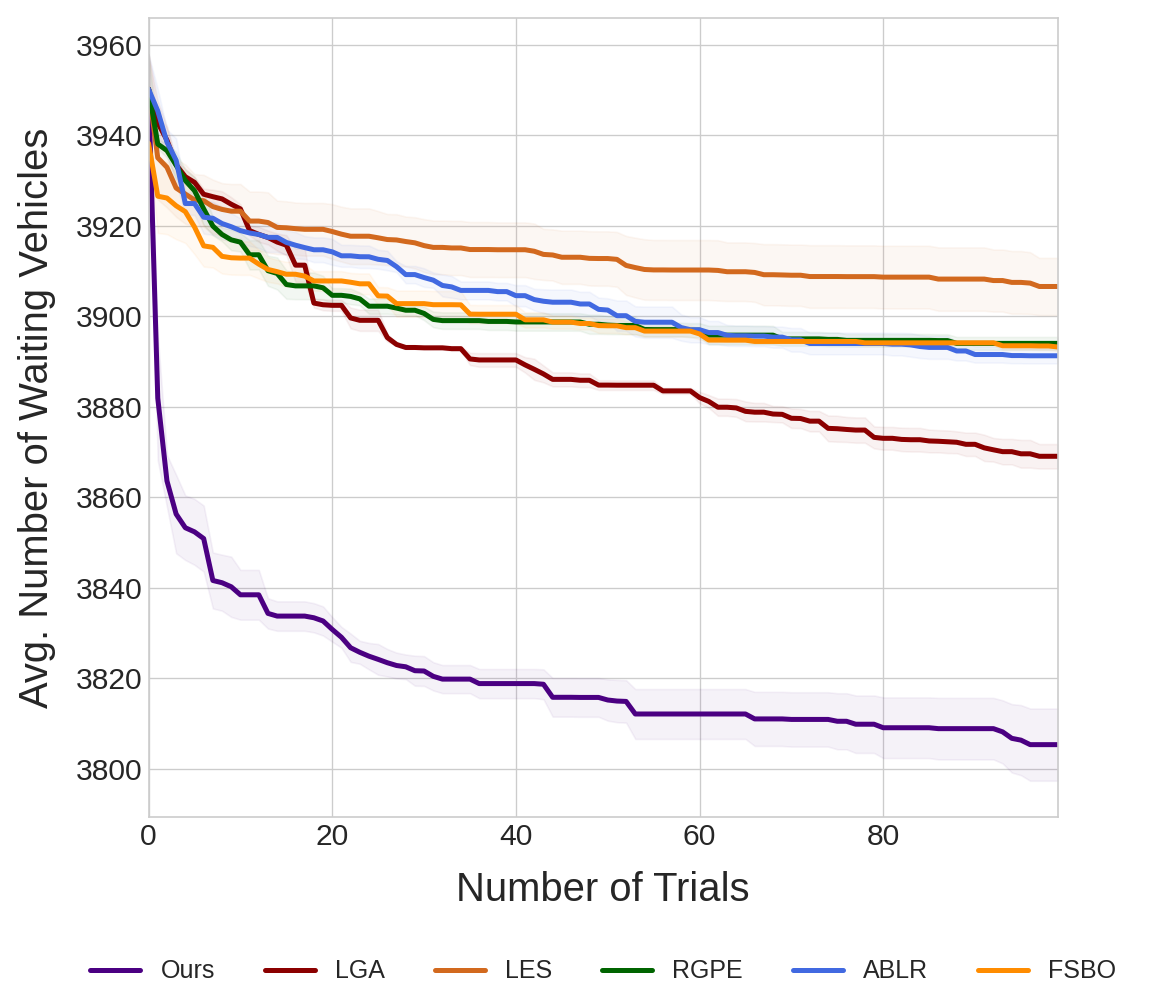}
         \caption{Phase allocation}
     \end{subfigure}     
\end{minipage} 
\caption{Experiments on Manhattan 28$\times$7 network}\label{figure:manhattan-large}
\end{figure*}
