# Supplementary material for: An Offline Meta Black-box Optimization Framework for Adaptive Design of Urban Traffic Light Management Systems
Source: arXiv:2408.07327 source file (2024-08-14)
Supplement: Supplementary file 3 [file data_collection.tex]

\subsection{Offline Data Collection}

For offline data collection, we use random sampling strategy for choosing designs to evaluate on different traffic patterns. While random sampling strategy may not be an optimal strategy, we can parallelize the data collection process. To this end, we compare the difference between other data collection techniques with our suggestion. Specifically, we use CMA-ES to collect the offline meta dataset and compare the execution time for collecting offline data and the performance of our method and baselines. Experiment is conducted on Grid\_3$\times$3 network. \Cref{table:data_collection} shows the results. As shown in the table, collecting the offline meta dataset using CMA-ES takes 20x times longer while leading to only a small fraction of increase in performance.

\begin{table}[t]
\centering
\caption{Comparison of different data collection strategies.}
\begin{tabular}{ccccc}
\toprule
\multirow{2}{*}{\textbf{Method}} & \multicolumn{4}{c}{\textbf{Average Number of Passing Vehicles ($\uparrow$)}}\\
\cmidrule{2-5}
  & Tue & Wed & Thu & \textbf{Overall}\\
\midrule
Fixed Time (veh/hr) & 16775 & 16072 & 19185 &\textbf{17344}\\
Ours (veh/hr)   & 17672 & 17735 & 19120 &\textbf{18176}\\
\midrule
Improvement (\%)	&	5.35	& 10.35 & -0.34 &\textbf{4.80}\\
\bottomrule
\end{tabular}
\label{table:data_collection}
\end{table}
